# Supplementary material for: Quantum-mechanics free subsystem with mechanical oscillators
Source: arXiv:2009.12902 ancillary file (2021-05-12)
Supplement: Supplementary file 1 [file 4_tone_BAE_SI.pdf]

# Quantum-mechanics free subsystem with mechanical oscillators: Supplementary Information

Laure Mercier de Lépinay, Caspar F. Ockeloen-Korppi, and Mika A. Sillanpää
*QTF Centre of Excellence, Department of Applied Physics, Aalto University, FI-00076 Aalto, Finland*

Matthew J. Woolley
*School of Engineering and Information Technology, UNSW Canberra, ACT, 2600, Australia*

## CONTENTS

I. Materials and Methods 1
A. Theoretical model 1
B. 4 pump tone Hamiltonian 1
1. Ideal BAE Hamiltonian 2
2. Variances 3
3. BAE noise spectra 4
4. Imprecision noise 5
C. Standard quantum limit of a single oscillator 6
D. Device details 7
E. Measurement electronics 7
F. Experimental calibrations 9
1. Effective couplings 9
2. Thermometry calibration 9
3. Temperature sweep 10
4. Phase calibrations 11
G. Error propagation 12

II. Supplementary Text 12
A. Force detection beyond full quantum limit 12

## I. MATERIALS AND METHODS

### A. Theoretical model

### B. 4 pump tone Hamiltonian

First, we will treat the system of two mechanical oscillators coupled to one cavity mode via a standard radiation-pressure type coupling. The cavity in the discussion below can be either the pump cavity or probe cavity, unless explicitly specified. The generic cavity mode is characterized by the annihilation and creation operators $a$, $a^\dagger$, and frequency $\omega_c$. The creation and annihilation operators for phonons are denoted $b_j$, $b_j^\dagger$, with $j = 1, 2$. The Hamiltonian is

$$H/\hbar = \omega_c a^\dagger a + \sum_{j=1,2} \omega_j b_j^\dagger b_j + \sum_{j=1,2} g_j \, a^\dagger a \left( b_j^\dagger + b_j \right) . \tag{S1}$$

Here, the frequencies of the two oscillators are $\omega_j$, and their single-photon coupling rates are $g_j$. The cavity is driven by four strong coherent tones that account for intra-cavity fields at the frequencies specified in the main text with amplitudes $|\alpha_{j\pm}|$ and phases $\theta_{j\pm}$. We will now write all equations in the interaction picture with respect to the time-independent Hamiltonian

$$H_0'/\hbar = (\omega_1 - \Omega) b_1^\dagger b_1 + (\omega_2 + \Omega) b_2^\dagger b_2 + \omega_c \, a^\dagger a. \tag{S2}$$

To simplify the notations, we denote the interaction-picture operators as their Schrödinger-picture counterparts. We follow a standard linearization procedure under strong pumping, and neglect for the moment terms oscillating at frequencies roughly equal to the average mechanical frequency, the mechanical frequency difference $\approx \pm|\omega_1 - \omega_2|$, and also those at higher frequencies. We obtain the linearized Hamiltonian

$$\begin{aligned} H/\hbar = \Omega \left( b_1^\dagger b_1 - b_2^\dagger b_2 \right) + g_1 \left[ \left( \alpha_{1-} b_1 + \alpha_{1+} b_1^\dagger \right) a^\dagger + \left( \alpha_{1-}^* b_1^\dagger + \alpha_{1+}^* b_1 \right) a \right] \\ + g_2 \left[ \left( \alpha_{2-} b_2 + \alpha_{2+} b_2^\dagger \right) a^\dagger + \left( \alpha_{2-}^* b_2^\dagger + \alpha_{2+}^* b_2 \right) a \right] . \end{aligned} \tag{S3}$$

Henceforth we will denote the effective complex-valued optomechanical coupling strengths as $G_{j\pm} = g_j \alpha_{j\pm}$.

In Eq. (S3) we notice the substantial practical benefit of the 4-tone protocol as compared to earlier work [4,11]. Since each process is driven by an independent pumping tone, the couplings $|G_{j\pm}|$ can be balanced for BAE measurements. Without this possibility, the single-photon couplings $g_1$ and $g_2$ need to match within a few percent; achieving this in practice is a matter of luck in device fabrication. Similarly, when generating entanglement, the balance of red and blue effective couplings, which controls the strength of the entanglement, can be tuned while maintaining the balance of coupling strength between mechanical oscillators. This is not possible with a 2-tone protocol and becomes possible with the present setup. Moreover, the frequencies of the positive and negative mass oscillator are $\pm\Omega$ and are therefore tunable, and they can be optimized with respect to $\kappa$ for entanglement generation. Another of the fundamental benefits of the 4-tone technique is the possibility to measure any of the four collective quadratures as discussed below.

### 1. *Ideal BAE Hamiltonian*

In order to describe the BAE measurement, we choose equal effective couplings $|G_{j\pm}| \equiv G$. The coupling part of the Hamiltonian Eq. (S3) becomes

$$H_c/\hbar = \frac{G}{2} a \left[ A_- X_- + A_+ X_+ + B_- P_- + B_+ P_+ \right] + \frac{G}{2} a^\dagger \left[ A_-^* X_- + A_+^* X_+ + B_-^* P_- + B_+^* P_+ \right] , \tag{S4}$$

where the coefficients are

$$\begin{aligned} A_- &= \exp(-i\theta_{1-}) + \exp(-i\theta_{1+}) - \exp(-i\theta_{2-}) - \exp(-i\theta_{2+}) \\ A_+ &= \exp(-i\theta_{1-}) + \exp(-i\theta_{1+}) + \exp(-i\theta_{2-}) + \exp(-i\theta_{2+}) \\ B_- &= i \Big[ - \exp(-i\theta_{1-}) + \exp(-i\theta_{1+}) + \exp(-i\theta_{2-}) - \exp(-i\theta_{2+}) \Big] \\ B_+ &= i \Big[ - \exp(-i\theta_{1-}) + \exp(-i\theta_{1+}) - \exp(-i\theta_{2-}) + \exp(-i\theta_{2+}) \Big] . \end{aligned} \tag{S5}$$

The coefficients $A_\pm$ and $B_\pm$ are complex-valued functions of all the pump tone phases. Hence, $H_c$ cannot generally be written as a simple coupling between a cavity quadrature and generalized mechanical quadrature, as would be required to describe a BAE measurement or properly define a QMFS. However, any linear combination of $X_\pm$ and $P_\pm$ can be measured with an appropriate choice of phases. With the choice $\theta_{1-} = \theta_{2+} = 0$ and $\theta_{1+} = \theta_{2-} \equiv \phi$, Eq. (S4) becomes

$$H_c/\hbar = 2G \left( e^{-i\phi/2} a + e^{i\phi/2} a^\dagger \right) \left( X_+ \cos\frac{\phi}{2} + P_- \sin\frac{\phi}{2} \right) . \tag{S6}$$

Other useful phase combinations are $\theta_{1-} = \theta_{2-} = 0$ and $\theta_{1+} = \theta_{2+} \equiv \theta$, which yields:

$$H_c/\hbar = 2G \left( e^{-i\theta/2} a + e^{i\theta/2} a^\dagger \right) \left( X_+ \cos\frac{\theta}{2} + P_+ \sin\frac{\theta}{2} \right) , \tag{S7}$$

and $\theta_{1-} = 0$, $\theta_{2-} = \pi$ and $\theta_{1+} = \theta_{2+} + \pi$, which yields:

$$H_c/\hbar = 2G \left( e^{-i\theta_{1+}/2} a + e^{i\theta_{1+}/2} a^\dagger \right) \left( X_- \cos\frac{\theta_{1+}}{2} + P_- \sin\frac{\theta_{1+}}{2} \right) , \tag{S8}$$

and $\theta_{1-} = 0$, $\theta_{2+} = \pi$ and $\theta_{1+} = \theta_{2-} + \pi$, which yields:

$$H_c/\hbar = 2G \left( e^{-i\theta_{1+}/2} a + e^{i\theta_{1+}/2} a^\dagger \right) \left( X_- \cos\frac{\theta_{1+}}{2} + P_+ \sin\frac{\theta_{1+}}{2} \right) . \tag{S9}$$

While we present above four constraints on the phases for each case corresponding to the phase combinations directly used in the experiment, note that only two constraints are actually required to define the subspace of measured collective quadratures. For example, setting $\theta_{1-} = \theta_{2+}$ and $\theta_{1+} = \theta_{2-}$, one obtains the Hamiltonian $H_c/\hbar = 2G\left(ae^{-i\psi} + a^\dagger e^{i\psi}\right)\left(X_- \cos\frac{\nu}{2} + P_+ \sin\frac{\nu}{2}\right)$ where $\psi = (\theta_{1+} + \theta_{1-})/2$ and $\nu = (\theta_{1+} - \theta_{1-})/2$, similar to Eq. (S6). The minimal phase requirements leading to the coupling of other subspaces are respectively: $\{\theta_{1-} = \theta_{2-};\ \theta_{1+} = \theta_{2+}\}$, $\{\theta_{2-} = \theta_{1-} + \pi;\ \theta_{1+} = \theta_{2+} + \pi\}$ and $\{\theta_{2+} = \theta_{1-} + \pi;\ \theta_{1+} = \theta_{2-} + \pi\}$.

The cavity quadrature to which the mechanical quadratures are coupled is rotated when the phases are modulated. However, phase-insensitive measurements of the cavity output power are not affected by these rotations.

In order to briefly illustrate the QMFS dynamics, we outline the equations of motion resulting from Eq. (1) in the main text, and with the coupling $H_c = 2\sqrt{2}\,G\,X_c X_+$, omitting dissipation terms:

$$\begin{aligned}
\dot{X}_c &= 0 \\
\dot{Y}_c &= -2\sqrt{2}\,G X_+ \\
\dot{X}_+ &= \Omega P_- \\
\dot{P}_+ &= -\Omega X_- - 2\sqrt{2}\,G Y_c \\
\dot{X}_- &= \Omega P_+ \\
\dot{P}_- &= -\Omega X_+
\end{aligned} \tag{S10}$$

We thus see that the quadratures $X_+$ and $P_-$ follow the dynamics of a free effective oscillator of frequency $\Omega$, being unperturbed by the cavity or the other quadratures.

### *2. Variances*

The total mechanical variance $\langle X^2\rangle^T$ corresponds to the mechanical thermal variance as seen by the BAE-measurement setup, that is, it results from the cryogenic cooling of oscillators and from auxiliary sideband-cooling if the latter is used.

We write the equations of motion following from Eq. (S3), including dissipation and fluctuations, as a linear system:

$$\frac{d}{dt} Z = \mathbf{A}\, Z + \mathbf{B}\, Z^{\text{in}}\,. \tag{S11}$$

Here, $Z = (X_+, P_-, X_-, P_+, X_c, P_c)^{\text{T}}$ is a vector of collective mechanical quadrature operators and cavity quadrature operators, $\mathbf{A}$ is the drift matrix found from the Hamiltonian evolution with the particular choice of $H_c$ determined by the phase configuration, and $Z^{\text{in}} = \left(X_+^{\text{in}}, P_-^{\text{in}}, X_-^{\text{in}}, P_+^{\text{in}}, X_c^{I,\text{in}}, P_c^{I,\text{in}}, X_c^{E,\text{in}}, P_c^{E,\text{in}}\right)^{\text{T}}$ is a vector of delta-correlated quadrature input noise operators. The labels $I$ and $E$ refer to the internal and external losses of the cavity respectively and the associated noise baths. The only nonzero correlators for these input noise operators are:

$$\begin{aligned}
\left\langle X_c^{I,\text{in}}(t) X_c^{I,\text{in}}(t')\right\rangle &= \left\langle P_c^{I,\text{in}}(t) P_c^{I,\text{in}}(t')\right\rangle = \delta(t-t') \\
\left\langle X_c^{E,\text{in}}(t) X_c^{E,\text{in}}(t')\right\rangle &= \left\langle P_c^{E,\text{in}}(t) P_c^{E,\text{in}}(t')\right\rangle = \delta(t-t') \\
\left\langle X_+^{\text{in}}(t) X_+^{\text{in}}(t')\right\rangle &= \left\langle X_-^{\text{in}}(t) X_-^{\text{in}}(t')\right\rangle = \left\langle P_+^{\text{in}}(t) P_+^{\text{in}}(t')\right\rangle = \left\langle P_-^{\text{in}}(t) P_-^{\text{in}}(t')\right\rangle = \delta(t-t').
\end{aligned} \tag{S12}$$

Thermal and quantum fluctuations are accounted for through the diffusion matrix $\mathbf{B}$, which may be represented in block matrix form as $\mathbf{B} = \left(\begin{array}{c|c} \mathbf{B}_{\text{mech}} & \mathbf{0}_{44} \\ \hline \mathbf{0}_{24} & \mathbf{B}_{\text{cav}} \end{array}\right)$ where

$$\mathbf{B}_{\text{mech}} = \sqrt{\gamma \langle X^2\rangle^T}\; \mathbb{I}_4, \qquad \mathbf{B}_{\text{cav}} = \begin{pmatrix} \sqrt{\kappa_I\left(n_c^I + \frac{1}{2}\right)} & 0 & \sqrt{\kappa_E\left(n_c^E + \frac{1}{2}\right)} & 0 \\ 0 & \sqrt{\kappa_I\left(n_c^I + \frac{1}{2}\right)} & 0 & \sqrt{\kappa_E\left(n_c^E + \frac{1}{2}\right)} \end{pmatrix}. \tag{S13}$$

Below we suppose that the external cavity modes are in the vacuum state, viz. $n_c^E = 0$ which is satisfied experimentally with adequate filtering of the transmission lines. The cavity thermal occupation is then related to the cavity internal bath drive amplitude as $n_c^T = n_c^I \kappa_I/\kappa$. The Lyapunov equation follows for the symmetrized covariance matrix $\mathbf{V} \equiv \frac{1}{2}\langle Z Z^{\text{T}} + Z^{\text{T}} Z\rangle$ as:

$$\frac{d}{dt}\mathbf{V} = \mathbf{A}\,\mathbf{V} + \mathbf{V}\,\mathbf{A}^{\text{T}} + \mathbf{B}\,\mathbf{B}^{\text{T}}. \tag{S14}$$

The elements of $\mathbf{V}$ denote all the symmetrized covariances of the quadratures, e.g. $V_{15} = \langle X_+ X_c \rangle$. Solving for the steady-state of Eq. (S14) allows us to evaluate the expected variances given a set of parameters. Alternatively the variances can be found from the integration of the spectra obtained by writing the Heisenberg-Langevin equations of motion. We therefore use the Lyapunov equation solution to confirm this alternative derivation of the variances and to investigate the system non-idealities where solving the equations of motion in the frequency domain becomes tedious.

### 3. *BAE noise spectra*

The noise spectra for the collective quadratures $X = X_\pm, P_\pm$ are obtained in a standard manner from the equations of motion:

$$S[\omega] \equiv \int_{-\infty}^{+\infty} \frac{d\omega'}{2\pi} \langle X[\omega] X[\omega'] \rangle. \tag{S15}$$

The spectral densities are connected to the variance, or total energy, of an arbitrary collective quadrature $X$ obtained from the spectral integration of $S[\omega]$ as

$$\langle X^2 \rangle = \frac{1}{2\pi} \int_{-\infty}^{+\infty} S[\omega]\, d\omega. \tag{S16}$$

Now, we assume that the pump phases are chosen such that the $X_+$ collective quadrature is measured:

$$H/\hbar = \Omega(X_+ X_- + P_+ P_-) + 2\sqrt{2} G X_c X_+. \tag{S17}$$

Quadratures perturbed by backaction are therefore expected to be $P_+$ and $X_-$ while we will show that $X_+$ and $P_-$ are not affected by backaction. Equations of motion are written from the Hamiltonian $H$, and taking Fourier transforms yields:

$$\begin{aligned}
X_+[\omega] &= \frac{\sqrt{\gamma}}{2} \sqrt{\langle X^2 \rangle^T} \left[ i\Big(\chi_m^+[\omega] - \chi_m^-[\omega]\Big) P_-^{\rm in}[\omega] \;+\; \Big(\chi_m^+[\omega] + \chi_m^-[\omega]\Big) X_+^{\rm in}[\omega] \right] \\
X_-[\omega] &= \frac{\sqrt{\gamma}}{2} \Bigg\{ -i\, 2\sqrt{2\kappa} G\, \chi_c[\omega] \sqrt{n_c^T + \frac{1}{2}} \Big(\chi_m^+[\omega] - \chi_m^-[\omega]\Big) X_c^{\rm in}[\omega] \\
&\qquad + \sqrt{\langle X^2 \rangle^T} \Big[ i\Big(\chi_m^+[\omega] - \chi_m^-[\omega]\Big) P_+^{\rm in}[\omega] \;+\; \Big(\chi_m^+[\omega] + \chi_m^-[\omega]\Big) X_-^{\rm in}[\omega] \Big] \Bigg\} \\
P_+[\omega] &= i\frac{\sqrt{\gamma}}{2} \Bigg\{ -i\, 2\sqrt{2\kappa} G\, \chi_c[\omega] \sqrt{n_c^T + \frac{1}{2}} \Big(\chi_m^+[\omega] + \chi_m^-[\omega]\Big) X_c^{\rm in}[\omega] \\
&\qquad + \sqrt{\langle X^2 \rangle^T} \Big[ -i\Big(\chi_m^+[\omega] + \chi_m^-[\omega]\Big) P_+^{\rm in}[\omega] \;-\; \Big(\chi_m^+[\omega] - \chi_m^-[\omega]\Big) X_-^{\rm in}[\omega] \Big] \Bigg\} \\
P_-[\omega] &= i\frac{\sqrt{\gamma}}{2} \sqrt{\langle X^2 \rangle^T} \left[ -i\Big(\chi_m^+[\omega] + \chi_m^-[\omega]\Big) P_-^{\rm in}[\omega] - \Big(\chi_m^+[\omega] - \chi_m^-[\omega]\Big) X_+^{\rm in}[\omega] \right].
\end{aligned} \tag{S18}$$

where we introduced the mechanical susceptibilities

$$\chi_m^\pm[\omega] = \frac{1}{\gamma/2 - i(\omega \mp \Omega)}, \tag{S19}$$

centered at $\pm\Omega$ and satisfying $\chi_m^+[-\omega] = (\chi_m^-[\omega])^*$, and the cavity susceptibility

$$\chi_c[\omega] = \frac{1}{\kappa/2 - i\omega}. \tag{S20}$$

From these expressions, we calculate the spectra $S[\omega]$ of the backaction-free quadratures and $S_*[\omega]$ of the quadratures affected by backaction in the experimentally relevant limit $\Omega \gg \gamma$:

$$\begin{aligned}
S[\omega] &= S_{X_+}[\omega] = S_{P_-}[\omega] = S_0[\omega] \langle X^2 \rangle^T \\
S_*[\omega] &= S_{X_-}[\omega] = S_{P_+}[\omega] = S_0[\omega] \left( \langle X^2 \rangle^T + 4C \frac{\kappa^2/4}{\kappa^2/4 + \omega^2} \left( n_c^T + \frac{1}{2} \right) \right)
\end{aligned} \tag{S21}$$

where $C = \frac{4G^2}{\kappa\gamma}$ is the common cooperativity of all probe tones and we introduced the sum of two Lorentzians centered at $\pm\Omega$:

$$S_0[\omega] = \frac{\gamma}{2}\left(\left|\chi_m^+[\omega]\right|^2 + \left|\chi_m^-[\omega]\right|^2\right) = \frac{\gamma/2}{(\omega+\Omega)^2 + \left(\frac{\gamma}{2}\right)^2} + \frac{\gamma/2}{(\omega-\Omega)^2 + \left(\frac{\gamma}{2}\right)^2}. \tag{S22}$$

The results in other cases of pump phases are analogous with different perturbed and unperturbed quadratures depending on the measured subspace. For the isolated QMFS quadratures ($X_+$ and $P_-$ in the calculation taken above), the variance in the thermal state is therefore

$$\langle X^2\rangle = \int_{-\infty}^{+\infty} S[\omega]\, d\omega = \langle X^2\rangle^T, \tag{S23}$$

whereas the conjugate quadratures are affected by quantum backaction (QBA) and by classical backaction due to the cavity's thermal population ($n_c^T$) calculated from the spectral integration of $S_*[\omega]$. The corresponding variances are written as

$$\begin{aligned} \langle X_*^2\rangle &\equiv \int_{-\infty}^{+\infty} S_*[\omega]\, d\omega = \langle X^2\rangle^T + n_{\rm qba} + n_{\rm cba}\,, \\ n_{\rm qba} &= 2C\frac{\kappa^2/4}{\kappa^2/4+\Omega^2} \approx 2C\,, \\ n_{\rm cba} &= 4C\frac{\kappa^2/4}{\kappa^2/4+\Omega^2}\, n_c^T \approx 4Cn_c^T, \end{aligned} \tag{S24}$$

where the approximations are valid in the experimentally relevant limit $\Omega \ll \kappa$.

### 4. *Imprecision noise*

The spectrum of the output photon flux, described by the annihilation operator $a_{\rm out} = a_{\rm in} - \sqrt{\kappa_E}\, a$, faithfully reproduces the measured mechanical quadrature spectrum on top of a cavity-noise background:

$$S_{\rm out}[\omega] = \frac{C\kappa\kappa_{\rm E}\gamma}{\omega^2 + \left(\frac{\kappa}{2}\right)^2} S[\omega] + \frac{\kappa\kappa_{\rm E}}{\omega^2 + \left(\frac{\kappa}{2}\right)^2} n_c^T + \frac{1}{2}, \tag{S25}$$

that is,

$$S_{\rm out}[\omega \simeq \pm\Omega] \simeq C\, R\, \gamma\, S[\omega] + R\, n_c^T + \frac{1}{2}\,, \tag{S26}$$

where we introduced the parameter $R$ to simplify the notations:

$$R \equiv \frac{\kappa\kappa_{\rm E}}{\Omega^2 + \left(\frac{\kappa}{2}\right)^2}\,. \tag{S27}$$

The $R$ parameter describes the transduction efficiency from the cavity to the output transmission line, and is different for the two cavities. Under the maximum efficiency, $R = 4$, but in the experiment the values of $R$ are 3.45 and 2.51 for the pump cavity and the probe cavity, respectively, because of modest internal losses and finite $\Omega/\kappa$ ratios. The recorded output spectrum after amplification with gain $\mathcal{A}$ and added noise $n_{\rm amp}$ is (32)

$$S_{\rm out}^{\mathcal{A}}[\omega] = \mathcal{A}\, S_{\rm out}[\omega] + (\mathcal{A}-1)n_{\rm amp} = \mathcal{A}\, C\, R\, \gamma\, S[\omega] + \mathcal{A}\, R\, n_c^T + \frac{1}{2}\mathcal{A} + (\mathcal{A}-1)n_{\rm amp}\,. \tag{S28}$$

This can be written as an inferred spectrum of the measured mechanical quadrature:

$$S^{\rm eff}[\omega] = \frac{1}{\mathcal{A}\, C\, R\gamma} S_{\rm out}^{\mathcal{A}}[\omega] = S[\omega] + S_{\rm imp}[\omega]\,, \tag{S29}$$

where the imprecision noise spectrum, in the approximation of high gain $\frac{\mathcal{A}-1}{\mathcal{A}} \simeq 1$, is

$$S_{\rm imp}[\omega] = \frac{1}{C\gamma} n_c^T + \frac{1}{CR\gamma}\left(n_{\rm amp} + \frac{1}{2}\right)\,. \tag{S30}$$

In the limit of very strong measurement $C \to \infty$, $S^{\text{eff}}[\omega]$ approaches the mechanical spectrum $S[\omega]$, with at resonance $S^{\text{eff}}[\pm\Omega] = \frac{2}{\gamma}\langle X^2\rangle^T$, and $S^{\text{eff}}[\pm\Omega] = \frac{1}{\gamma}$ if the mechanical oscillators are in their quantum ground state.

$S[\omega]$ or $S^{\text{eff}}[\omega]$ given in units of quanta/Hz do not allow the most transparent interpretation. It is convenient to present the mechanical spectrum in a dimensionless form, such that the resonant value corresponds to zero-point energy:

$$\begin{aligned} S_0^n[\omega] &= \frac{\gamma}{2} S[\omega]\,, \\ S^n[\omega] &= \frac{\gamma}{2} S^{\text{eff}}[\omega]\,, \end{aligned} \tag{S31}$$

In the ground state, $S_0^n[\pm\Omega] = \frac{1}{2}$. The inferred dimensionless mechanical spectrum is written as

$$\begin{aligned} S^n[\omega] &= \frac{\gamma}{2} S[\omega] + S^n_{\text{imp}}[\omega]\,, \\ S^n_{\text{imp}}[\omega] &= \frac{1}{2C} n_c^T + \frac{1}{2CR}\left(n_{\text{amp}} + \frac{1}{2}\right)\,. \end{aligned} \tag{S32}$$

The resonant values lead to the definition of effective mechanical variances:

$$\begin{aligned} \langle X^2_{\text{eff}}\rangle &\equiv S^n[\pm\Omega] = \langle X^2\rangle^T + n_{\text{imp}}\,, \\ n_{\text{imp}} &= \frac{1}{2CR}\left(n_{\text{amp}} + \frac{1}{2}\right) \approx \frac{1}{8C}\left(n_{\text{amp}} + \frac{1}{2}\right)\,. \end{aligned} \tag{S33}$$

### C. Standard quantum limit of a single oscillator

Let us recall the analysis of a continuous monitoring of the position of a single oscillator. Such a measurement is carried out, for example, by probing a cavity-optomechanical system at the resonant frequency of the cavity. The probing tone enhances conversion processes that imprint the mechanical spectrum around each of the optomechanical sidebands frequencies $\omega_c \pm \omega_1$. This measurement is not backaction-evading: the mechanical oscillator is driven by QBA. In order to derive the fundamental limit on position measurement, we suppose that the cavity output spectrum carrying the mechanical information encoded at the sideband frequencies is measured with a noiseless phase-sensitive amplifier. The single-oscillator spectrum has a double-Lorentzian form $S_0[\omega]$ in Eq. (S22) where $\Omega$ is replaced by the mechanical frequency $\omega_1$. We consider the bad-cavity limit $\omega_1 \ll \kappa$. We assume that the oscillator is in the ground state, $\langle X^2\rangle = \frac{1}{2}$, disregard the cavity noise $n_c^T$ and cavity losses, viz. $\kappa = \kappa_E$. Further, we assume that only the $Y$ quadrature of the output field is detected, which mitigates the noise in the $X$ quadrature that does not contain information. The inferred mechanical variances are

$$\begin{aligned} S^n[\omega] &= \frac{\gamma}{4} S_0[\omega] + S^n_{\text{qba}}[\omega] + S^n_{\text{imp}}[\omega]\,, \\ S^n_{\text{qba}}[\omega] &= n_{\text{qba}} \frac{\gamma}{2} S_0[\omega]\,, \\ S^n_{\text{imp}}[\omega] &= \frac{1}{16C}\,, \\ n_{\text{qba}} &= C\,. \end{aligned} \tag{S34}$$

The sum of QBA and of the imprecision due to the quantum noise of the output field is minimized at frequency $\omega$ for the SQL cooperativity $C^{\text{sql}} = \frac{1}{2\sqrt{2\gamma S_0[\omega]}}$ and is:

$$\begin{aligned} S^n_{\text{add,sql}}[\omega] &= \frac{\gamma}{2} C^{\text{sql}} S_0[\omega] + \frac{1}{16 C^{\text{sql}}} = \frac{\sqrt{\gamma S_0[\omega]}}{2\sqrt{2}}\,, \\ S^n_{\text{sql}}[\omega] &= \frac{\gamma}{4} S_0[\omega] + S^n_{\text{add,sql}}[\omega]\,. \end{aligned} \tag{S35}$$

The resonant values are $S^n[\pm\omega_1]$

$$\begin{aligned} \langle X^2_{\text{eff}}\rangle &= \frac{1}{2} + n_{\text{qba}} + n_{\text{imp}} \\ n_{\text{qba}} &= C \\ n_{\text{imp}} &= \frac{1}{16C} \end{aligned} \tag{S36}$$

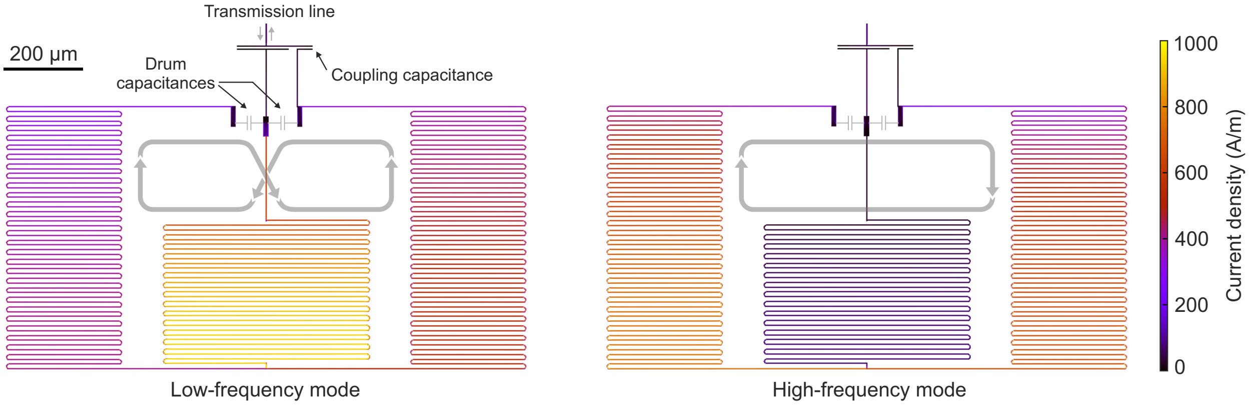


FIG. S1. *Cavity design.* The electromagnetic simulation shows the distribution of current of the two cavity modes at their respective resonance frequencies. The two drum membranes are replaced in this simulation by equivalent ideal capacitances.

The best force sensitivity is reached when the force is modulated at the resonant frequency; hence the resonant case is the most interesting. On resonance, the sum of QBA and of the imprecision due to quantum noise of the output field is minimized at the SQL cooperativity $C^{\rm sql} = \frac{1}{4}$ and gives

$$\begin{aligned} \langle X_{\rm eff}^2 \rangle^{\rm sql} &= 1 \\ n_{\rm add,sql} &= n_{\rm qba}^{\rm sql} + n_{\rm imp}^{\rm sql} = \frac{1}{2} \end{aligned} \tag{S37}$$

That is, the added noise on the mechanical resonance equals the zero-point noise (half a quantum), and the total noise is twice the zero-point noise. The latter case has been referred to in the literature as the *full quantum limit*, which is the special case of the SQL where the oscillator would be in its ground state of motion, were it not driven by backaction. The full quantum limit is much more difficult to reach than the SQL since it can only be attained if the oscillator is cooled very close to the ground state.

## D. Device details

The cavity structure supports two lowest frequency modes in the range 4.5 GHz ... 7.5 GHz depending on the drum capacitances. The currents in the modes flow either symmetrically or antisymmetrically in two circuit loops as displayed in Fig. 1B in the main text. The current distributions corresponding to each cavity mode are detailed further in Fig. S1.

The mechanical oscillators are circular aluminum drums of diameters 20 $\mu$m (oscillator 1) and 15 $\mu$m (oscillator 2). The effective masses are, respectively, around 135 pg and 75 pg. The drum membranes are separated from a counter electrode beneath by a vacuum gap of $\sim$ 90 nm. Within the geometry of the device illustrated in Fig. S1, the single-photon optomechanical couplings to the low-frequency cavity mode (resonating at 4.98 GHz) are $g_{0,11} = 70$ Hz and $g_{0,12} = 49$ Hz and the single-photon optomechanical couplings to the high-frequency mode (resonating at 6.62 GHz) are $g_{0,21} = 44$ Hz and $g_{0,12} = 30$ Hz. We choose the better coupled, low-frequency cavity mode to be the pump cavity because stronger effective couplings are needed for pumping rather than for probing.

The input tones are applied via the coupling capacitance between the cavities and a transmission line. The output signal also leaks out via this route. The design of the split coupling capacitance is carefully chosen such that the electric field in either cavity mode couples in a similar manner to the measurement line.

## E. Measurement electronics

For generation of the microwave tones, we used a combination of ten PLL chips Texas Instruments LMX2594 15-GHz Wideband PLLatinum RF Synthesizer (33). They are locked by a 200 MHz reference derived from a high-purity RF source. We tested power stability of $\pm 0.02$ dB, and phase stability $\pm 0.5$ degrees, in ca. 24 hours as shown in Fig. S2. These numbers are well sufficient for the present purpose, and noticeably better than those for mainstream

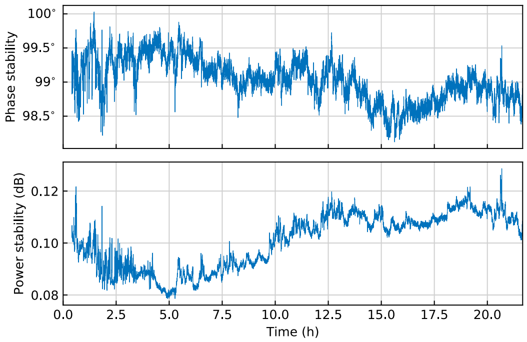


FIG. S2. *Stability of PLL microwave source.* Phase between two channels (up), and power difference between two channels (down).

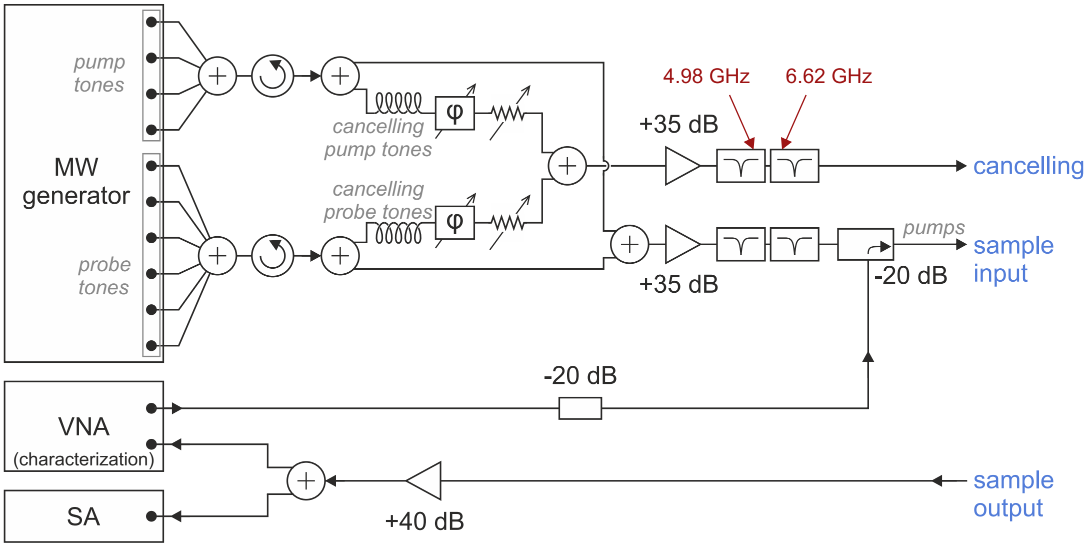


FIG. S3. *Room-temperature microwave electronics.* Ten phase-locked microwave sources are combined into a single input line. Two cancelling setups, one for either cavity, involving a phase shifter, a tunable attenuator and a length of cable, allow for interferometric cancelling of the strong microwave tones before the cryogenic amplifier.

sources. Notice that all ten tones are in use in the pump plus probe BAE tomography displayed in Fig. 3D in the main text. The two cooling tones, however, do not need to be phase stable.

Any electrical noise injected at the sideband frequencies would drive the mechanical oscillators and cause a heating detrimental to the generation of low-noise states. Therefore, we insert two cascaded tunable notch filters on each input line: WTRCJV6-4000-5000-3-22-30SS and WTRCJV6-5000-6000-3-20-30SSK, from Wainwright Instruments GmbH, to filter phase noise from the sources. The central frequency of these filters is parked at the frequency of either cavity, and they both attenuate by $-40$ dB with a $-3$ dB-bandwidth of about 3 MHz.

The electrical length of the input line and the cancelling line are matched at room temperature such that sufficient cancelling can be obtained for the tones applied to either cavity.

The added noise, $n_{\mathrm{amp}}$ from Eq. (S28), is different for the two cavities due to frequency dependence of the system noise (and notably, of the amplifier). The frequency dependence arises in the cryogenic amplifier, and is also contributed by a frequency dependent attenuation between the sample and the amplifier. We obtain $n_{\mathrm{amp}} \simeq 12$ and $n_{\mathrm{amp}} \simeq 25$ for the pump and probe cavities, respectively. It is not clear why the latter displays a substantially higher noise.

### F. Experimental calibrations

The discussion below holds for either the pump tones applied to the pump cavity, or for the probe tones applied to the auxiliary cavity. When the distinction is needed, it is explicitly stated. The subscripts $i = 1, 2$ refer to the two mechanical oscillators. We denote the calibration coefficients to be determined experimentally by calligraphic capital fonts.

#### 1. *Effective couplings*

We drive oscillator $j$ using a sideband-resonant red tone at the angular frequency $\omega_c - \omega_j$. The square of the steady-state field amplitude at the driven frequency is proportional to the generator power setting $P_j$ through a chain of attenuation stages which we incorporate into a proportionality constant $\mathcal{J}_j$, such that the squared effective optomechanical probe coupling is written as

$$G_{j-}^2 = \mathcal{J}_j P_j \,, \tag{S38}$$

The corresponding optical damping rate is

$$\gamma_{\rm opt,j} = \frac{4G_{j-}^2}{\kappa} = \frac{4\mathcal{J}_j P_j}{\kappa} \,. \tag{S39}$$

We linearly fit the optomechanical damping rate as a function of generator power, obtaining

$$\gamma_{\rm opt,i} = \mathcal{L}_j P_j \,, \tag{S40}$$

and comparison with Eq. (S39) yields the calibration coefficient:

$$\mathcal{J}_j = \frac{\mathcal{L}_j \kappa}{4} \,. \tag{S41}$$

The cooperativity is obtained the same way:

$$C_j = \frac{\gamma_{\rm opt,i}}{\gamma_j} = \frac{\mathcal{L}_j}{\gamma_j} P_j \,. \tag{S42}$$

We balance the effective couplings for the red-detuned BAE tones based on the above procedure, so that e.g. when sweeping the cooperativity, the generator channels are maintained at a fixed power ratio. Below, we predominantly work with the power applied to the oscillator 1, denoting it as $P \equiv P_1$.

The theoretical predictions for the variances and imprecision are evaluated using Eq. (S42) in Eqs. (S24) and (S33).

If the powers of the BAE tones are not balanced, backaction is visible as a change of mechanical linewidth, and as heating or cooling. It is thus necessary to follow both the linewidth and mechanical variance as displayed in Fig. 2 in the main text. The requirement of balancing of effective couplings becomes more stringent towards increasing cooperativity. At $C \ll 1$, there is little backaction, and for the sake of successful BAE, power balance is not important. At the highest $C \sim 5$ used in the BAE measurements, the effective couplings need to match within $\sim 2$ % $\sim 0.2$ dB, and pump phases within $\sim 5$ %. Given the stability of phase and power quoted in Section III, the requirements are well satisfied.

#### 2. *Thermometry calibration*

We calibrate the area of the mechanical peaks in the probe output spectrum at a given probe generator power and at a known mechanical variance (corresponding to a known cryostat temperature). This allows to infer the mechanical variance at another generator power by simple scaling with the probe power. The area is obtained from a Lorentzian fit to either mechanical peak, and summing the areas of the two peaks. For this calibration, we do not apply auxiliary sideband-cooling and we deal with mechanical variances associated with cryogenic cooling alone, which we denote $\langle X^2 \rangle^{T,0}$ as in the main text to distinguish from the effective variances $\langle X^2 \rangle^{T}$ which might differ from the latter if auxiliary sideband-cooling is employed.

The mechanical peak contribution to the measured probe output spectrum is given by the first term in Eq. (S28):

$$S_{\rm out}^{\mathcal{A},\rm m}[\omega] = \mathcal{A} R C \gamma S[\omega] \,, \tag{S43}$$

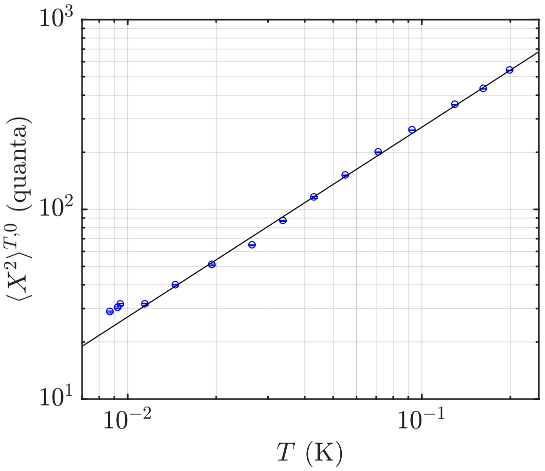


FIG. S4. *Thermal calibration.* Phonon numbers when changing the cryostat temperature $T$ in the four-tone BAE configuration, calibrated by integrating two peaks that appear about the cavity frequency.

and similarly we obtain the photon flux corresponding to the mechanical peak

$$N_{\text{out}}^{\mathcal{A},\text{m}} = \mathcal{A}RC\gamma\langle X^2 \rangle \,, \tag{S44}$$

which allows for the inference of $\langle X^2 \rangle$ once sufficient information on the parameters $\mathcal{A}$, $C$, $R$, and $\gamma$ is available. We operate at a known bath temperature where, according to the thermal calibration from Fig. S4 the system is properly thermalized at the cryostat temperature. The collective quadrature variance is therefore known: for example, $\langle X^2 \rangle^{T,0} \simeq 30$ at the calibration temperature $T \simeq 11$ mK.

We vary the generator power, and fit a straight line to the peak area, obtaining the calibration coefficient $\mathcal{N}$ that links the power and peak area (Fig. S5):

$$N_{\text{out}}^{\mathcal{A},\text{m}} = \mathcal{N}P \,. \tag{S45}$$

By combining Eqs. (S44) and (S45) at $\langle X^2 \rangle = \langle X^2 \rangle^{T,0}$ we can solve for the product

$$\mathcal{A}CR = \frac{\mathcal{N}P}{\gamma\langle X^2 \rangle^{T,0}} \,. \tag{S46}$$

which, after insertion back into Eq. (S44), gives the thermometer calibration:

$$n = \frac{N_{\text{out}}^{\mathcal{A},\text{m}}}{\mathcal{N}P}\langle X^2 \rangle^{T,0} \,. \tag{S47}$$

We also obtain the gain:

$$\mathcal{A} = \frac{\mathcal{N}}{\mathcal{L}R\langle X^2 \rangle^{T,0}} \,. \tag{S48}$$

The spectra $S^{\text{eff}}[\omega]$, as presented in Figs. 2B,C in the main text, are also obtained from the calibration. We substitute the factor $\mathcal{A}CR\gamma$ from Eq. (S46) to Eq. (S29), obtaining

$$S^{\text{eff}}[\omega] = \frac{S_{\text{out}}^{\mathcal{A}}[\omega]}{\mathcal{N}P}\langle X^2 \rangle^{T,0} \,. \tag{S49}$$

### *3. Temperature sweep*

We find the variance at the thermal equilibrium $\langle X^2 \rangle^{T,0}$ in Eq. (S47) using a standard temperature sweep in the complete four-tone BAE configuration. Mechanical frequencies are slightly temperature-dependent, and thus we first

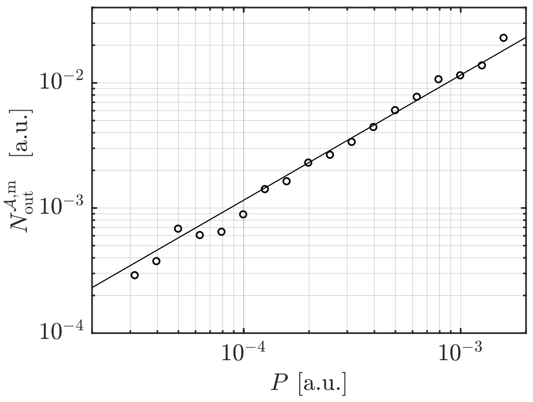


FIG. S5. *Probe power calibration.* The solid line is a fit according to Eq. (S44). For discussion, see text.

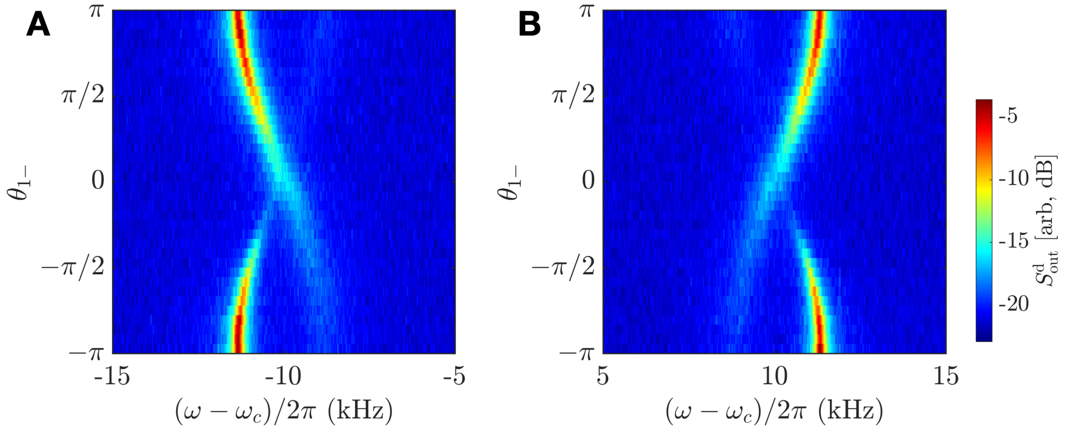


FIG. S6. *Non-BAE phases.* The pump cavity output spectra (a.u.) when the pump phase $\theta_{1-}$ is adjusted such that BAE conditions are met only when $\theta_{1-}=0$. $\Omega/2\pi = 10$ kHz, $C \simeq 2.0$. **(A)** Spectrum to the left from cavity. **(B)** Spectrum to the right from cavity.

record the frequencies using a single weak red tone, and correct the pump frequencies accordingly in order to maintain a constant $\Omega$ (see the pumping scheme in Fig. 1 in the main text). The powers described by the $P$ parameter are adjusted such that $C \ll 1$. Technical heating at these powers is expected to negligible, although the analysis does not depend on this assumption since Eq. (S47) connects $\langle X^2\rangle^{T,0}$ to a given $P$. Beforehand, we adjust the pump phases such that the measurement is BAE, even though at $C \ll 1$ the correct phase relationship is nearly irrelevant.

We run the sweep using the auxiliary cavity, because this cavity is the basis for accurate tomography results. We display the temperature sweep in Fig. S4. As seen in the figure, there is a slight thermal decoupling below $T \simeq 11\,$mK.

### *4. Phase calibrations*

In order to reach a BAE measurement, either in the pump or probe cavities, the phases of the tones need to be properly adjusted. We set all other phases to fixed values, and scan $\theta_{1-}$. The BAE condition is easily identified from the data (Fig. S6) as the phase where the peaks become Lorentzian.

In a thermal state, all the quadrature variances are equal, and we can identify this set of phases as measuring $X_+$, and conveniently label all phases equal to zero. Departures from this phase combination, according to the recipe shown e.g. Fig. 3A in the main text, allows one to move between the quadratures.

When preparing for the tomography via the auxiliary cavity, a similar phase calibration is carried out with the auxiliary cavity while the tones applied to the pump cavity are switched off. Notice that when a nontrivial state

is prepared via the pump cavity, we cannot, even after this calibration, know which generalized quadrature we are measuring. For example, there is an unknown phase offset in $\phi$ in Eq. (2) in the main text. However, we know even in this case *between which* quadratures we are moving when the probe phases are scanned in an appropriately correlated fashion.

### G. Error propagation

Here we discuss the error estimates for the two-mode squeezing measurement based on the calibration Eq. (S47). We thus have to find uncertainties on parameters $N_{\rm out}^{\mathcal{A},\rm m}$, $\mathcal{N}$, and $\langle X^2\rangle^{T,0}$. Then we use uncorrelated error propagation to find out the final error estimates. All the error bars in this work are $2\sigma$ (95 %) confidence limits.

We estimate the temperature measurement error by comparing two calibrated $RuO_2$ sensors attached next to one another in the cryostat in the same cooldown. These differ by 5 % to 10% from one another near the base temperature, giving an estimate $\pm 5\%$ for the temperature error. From the thermal sweep Fig. S4 we obtain the uncertainty for the slope $\pm 3$ %. These two propagate to the uncertainty in $\delta\langle X^2\rangle^{T,0}/\langle X^2\rangle^{T,0} \simeq \pm 6$ %, or $\delta\langle X^2\rangle^{T,0} \simeq \pm 2$ quanta. Statistical uncertainty in extracting the thermal peak area in $\langle X^2\rangle^{T,0}$ is negligible.

From the power fit as in Fig. S5 we get $\delta\mathcal{N}/\mathcal{N} \simeq 6$ %.

The uncertainty $\delta N_{\rm out}^{\mathcal{A},\rm m}$ in the probe peak areas, examples of which are shown in Fig. 4B in the main text, is evaluated as follows. We compute the standard error of the residual between the data and the fitted double-peaked Lorentzian profile $S_0[\omega]$;

$$\delta N_{\rm out}^{\mathcal{A},\rm m} = \frac{2}{\sqrt{N}}\sqrt{\sum_k^N \left[N_{\rm out}^{\mathcal{A},\rm m}[k] - S_0[k]\right]^2}\,, \tag{S50}$$

The summation is over the frequency points $k$ (total number $N$) in a single curve. Equation (S50) amounts to $\delta N_{\rm out}^{\mathcal{A},\rm m}/N_{\rm out}^{\mathcal{A},\rm m} \simeq \pm 2...5$ % depending on the phase.

The uncertainties on $\mathcal{N}$ and $\langle X^2\rangle^{T,0}$ are hence somewhat dominating the error over that in $N_{\rm out}^{\mathcal{A},\rm m}$.

## II. SUPPLEMENTARY TEXT

### A. Force detection beyond full quantum limit

We discuss the detection of a narrowband force applied resonantly to oscillator 1 at the center frequency $\omega_d \approx \omega_1$,

$$f_0(t) = f_s(t)\sin(\omega_d t) + f_c(t)\cos(\omega_d t) = \frac{f_x(t)\exp(-i\omega_d t) + f_x^*(t)\exp(i\omega_d t)}{\sqrt{2}}\,, \tag{S51}$$

where $f_s(t) = i\left[f_x^*(t) - f_x(t)\right]/\sqrt{2}$ and $f_c(t) = \left[f_x(t) + f_x^*(t)\right]/\sqrt{2}$ are the quadrature amplitudes. The force term added to the Hamiltonian is $H_F/\hbar = f_0(t)x_1$, and in the interaction picture

$$H_F/\hbar = f(t)\left[b_1 e^{i(\omega_1-\Omega)t} + b_1^\dagger e^{i(\omega_1-\Omega)t}\right] = f_y(t)b_1 + f_y^*(t)b_1^\dagger\,, \tag{S52}$$

where $f(t) = x_{\rm zp}f_0(t)$, $x_{\rm zp}$ denoting zero-point position fluctuations for oscillator 1, and $f_y(t) = f(t)\exp[-i(\omega_1-\Omega)t]$. Note that the content of the force $f_0$ at frequencies $\pm\omega_1$ is encoded in $f_y$ in the frequency components $\pm\Omega$ (and $\pm 2\omega_1 \pm \Omega$). The complex quantity $f_y$ contains information on both quadratures $f_c$ and $f_s$ of the force: by measuring both its real and imaginary part without ambiguity, one can infer both quadratures of the applied force. The equations of motion of $X_\pm$ and $P_\pm$ each receive an additional term due to the application of the force:

$$\begin{aligned} X_\pm[\omega] &\to X_\pm[\omega] - i\Big\{\chi_m^+[\omega]F_y[\omega] - \chi_m^-[\omega]F_y^*[\omega]\Big\}/\sqrt{2}\,,\\ P_\pm[\omega] &\to P_\pm[\omega] + \Big\{\chi_m^-[\omega]F_y[\omega] + \chi_m^+[\omega]F_y^*[\omega]\Big\}/\sqrt{2}\,, \end{aligned} \tag{S53}$$

where $F_y[\omega]$ is the Fourier transform of $f_y(t)$. The $\chi_m^\pm$ susceptibilities evaluated for $\omega \simeq +\Omega$ are:

$$\chi_m^+[\Omega] \approx \frac{2}{\gamma}, \qquad \chi_m^-[\Omega] \approx \frac{i}{2\Omega} \ll \chi_m^+[\Omega]\,. \tag{S54}$$

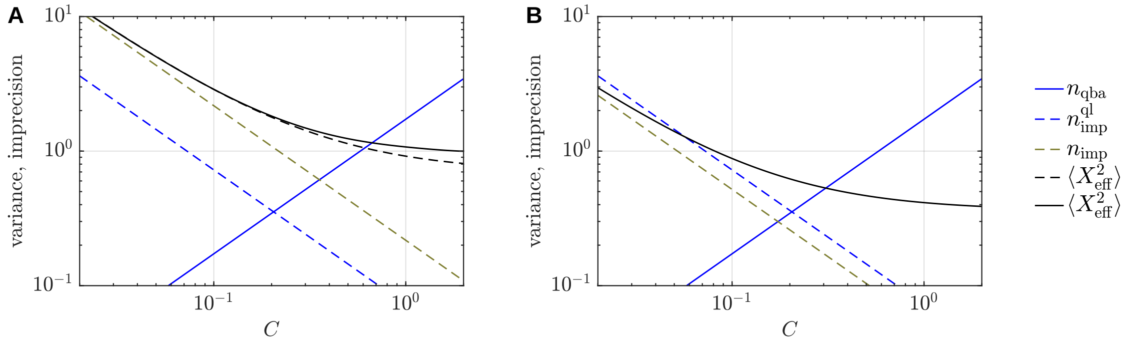


FIG. S7. *Prospects for surpassing the full quantum limit of continuous force detection.* The lines are as in Fig. 2B,C in the main text. **(A)** Low-noise amplifier with $n_{\mathrm{add}} = 1$, and near-ground state cooled oscillators with $\langle X^2\rangle^T = 0.7$, at $\gamma/2\pi = 20$ kHz. Solid black line for $\langle X_{\mathrm{eff}}^2\rangle$ is with technical heating, and the dashed white line is without technical heating. **(B)** Utilizing squeezing. We suppose a nearly noiseless phase-sensitive amplifier with $n_{\mathrm{add}} = 0.2$. The input microwave noise is two-mode squeezed by 5 dB, and the oscillators are two-mode squeezed by 1.4 dB.

Therefore, the motional quadratures at $+\Omega$ are essentially modified by:

$$\begin{aligned} X_\pm[\Omega] &\to X_\pm[\Omega] - \frac{i\sqrt{2}}{\gamma} F_y[\Omega]\,, \\ P_\pm[\Omega] &\to P_\pm[\Omega] - \frac{\sqrt{2}}{\gamma} F_y^*[\Omega]\,. \end{aligned} \tag{S55}$$

Depending on if $X_+$ or $P_-$ is measured (within a QMFS formed by both these collective quadratures), the corresponding quantity in Eq. (S55) is mapped into the output field in a similar manner. This allows for a full tomography of a force applied near-resonantly on one of the oscillators, even if the cavity output signal is affected by unknown phase shifts along the detection lines. Neither $X_+$-measurements nor $P_-$-measurements are affected by QBA noise, and since these collective quadratures form the QMFS, both can be probed without affecting the other one.

We now extrapolate the possibility to beat the full quantum limit in the four-tone BAE detection, namely $\langle X_{\mathrm{eff}}^2\rangle < 1$, in our setup. To reach the full quantum limit, the oscillators need to be very close to the ground state, $\langle X^2\rangle^T \simeq \frac{1}{2}$ as seen in Eq. (S33). The value of $\langle X^2\rangle^T$ is set by the competition between technical noise and sideband cooling. It is still possible to further reduce $\langle X^2\rangle^T$ in the current sample, down to $\sim 0.7$. However, at stronger sideband cooling, $\gamma$ increases such that sufficient cooperativity cannot be reached (and imprecision would become the bottleneck) before the microwave power becomes excessively high and technical heating due to BAE detection would start to limit $\langle X^2\rangle^T$. We have not thoroughly tested which sideband cooling power would offer the "sweet spot", but we believe it is rather close to the situation in Fig. 2C in the main text. The next step to improve the experiment is likely to reduce the imprecision noise by using near-quantum limited Josephson parametric amplifiers (JPA).

We now assume that such a low-noise amplifier is used. We take the situation of Fig. 2C in the main text, except that we assume that the oscillators are initially cooled down closer to their ground state, viz. $\langle X^2\rangle^T = 0.7$ which has been experimentally reached in our system in spite of technical heating. We then show in Fig. S7A the predicted noise contributions. Because of larger mechanical linewidth due to stronger sideband cooling, technical heating would arise at a smaller cooperativity, which is taken into account in this calculation. As seen in Fig. S7A, the effective measurement noise can attain the full quantum limit solely by adopting a JPA, which thus seems experimentally within reach.

To go beyond, an interesting direction is to employ phase-sensitive correlations, with the idea of reducing the variances in the measurement below the vacuum noise level:

(1) *nearly noiseless phase-sensitive amplification* allows to eliminate $n_{\mathrm{amp}}$ in Eq. (S32).

(2) *Two-mode squeezing of the incoming field* allows to eliminate the "1/2" in Eq. (S32) that can be associated to shot noise of the incoming field. More precisely, correlators of the input noises $X_c^{\mathrm{in}}$ and $P_c^{\mathrm{in}}$ can be different from that in Eqs. (S12), falling below the vacuum level.

(3) *Two-mode squeezing (entanglement) of the mechanics*, as we have demonstrated in this work, will push the variance $\langle X^2 \rangle < 1/2$ in Eq. (S16).

Ideally, implementing the above allows for noiseless detection, $\langle X_{\mathrm{eff}}^2 \rangle \to 0$. In practice, there are substantial limitations to the amount of squeezing, or to the added noise of a phase-sensitive amplifier. In Fig. S7B, we show the effective noise when all (1) - (3) are utilized, supposing (2) and (3) are independent. The parameters are all realistic and experimentally reached, and the mechanical two-mode squeezing is similar to the one demonstrated in this work. Notice that due to (2), imprecision is below the quantum-limited imprecision. The amount of mechanical two-mode squeezing is the limiting factor for the effective noise in the proposed situation. We see that surpassing the full quantum limit by a factor of two is also realistically within reach using the techniques discussed in this work.
